# Supplementary material for: Learning Navigation Costs from Demonstration in Partially Observable Environments
Source: arXiv:2002.11637 source file (2020-02-26)
Supplement: Supplementary file 1 [file Appendix.tex]

\section{Supplementary Material}
\subsection{Derivation of log-odds ratio} 
If the observation model is a sigmoid funtion parameterized by $\theta_1$:
\begin{equation}
\begin{aligned}
p(z_t|\hat{m};\theta_1) &:= 
\begin{cases}
    \sigma(\theta_1),& \text{if } z_t = \hat{m}\\
    \sigma(-\theta_1), & \text{if } z_t \neq \hat{m}
\end{cases} \\
&= \sigma((2z_t-1)(2\hat{m}-1)\theta_1) \;,
\end{aligned}
\end{equation}
we can simplify the log-odds ratio of the observation model as follows,
\begin{equation}
\begin{aligned}
\ln \frac{p(z_t|\hat{m}=1)}{p(z_t|\hat{m}=0)} &= \ln \frac{\sigma((2z_t-1)\theta_1)}{\sigma(-(2z_t-1)\theta_1)} \\
&= \ln \frac{1+e^{(2z_t-1)\theta_1}}{1+e^{-(2z_t-1)\theta_1}} \\
&= \ln(e^{(2z_t-1)\theta_1}(1+e^{-(2z_t-1)\theta_1})) \\
&\;\; - \ln (1+e^{-(2z_t-1)\theta_1}) \\
&= (2z_t-1)\theta_1 \;.
\end{aligned}
\end{equation}
Given a history of observations $z_{1:t}$, the log-odds ratio of the occupancy probability is
\begin{equation}
\begin{aligned}
\lambda(\hat{m} \mid z_{1:t}) &:= \ln \frac{p(\hat{m}=1 \mid z_{1:t})}{p(\hat{m}=0 \mid z_{1:t})} \; \\
&= \ln \frac{p(z_t \mid \hat{m}=1)p(\hat{m}=1 \mid z_{1:t-1})}{p(z_t \mid \hat{m}=0)p(\hat{m}=0 \mid z_{1:t-1})} \\
&= \lambda(\hat{m} \mid z_{1:t-1}) + \ln \frac{p(z_t \mid \hat{m}=1)}{p(z_t \mid \hat{m}=0)}  \\
&= \lambda(\hat{m}) + \sum_{\tau=1}^t \ln \frac{p(z_{\tau} \mid \hat{m}=1)} {p(z_{\tau} \mid \hat{m}=0)} \; \\
&= \lambda(\hat{m}) + \sum_{\tau=1}^t (2z_{\tau}-1)\theta_1
\end{aligned}
\end{equation}
with some prior $\lambda(\hat{m})$. 

\subsection{Proof of Proposition 1}
\label{app:a}
%We present a proof for Proposition 1 as follows.
\begin{proof}
 Assuming that the optimal path from $x_t$ to $x_g$ is unique, the DP algorithm computes the optimal cost-to-go at every state (at least propagated from $x_g$ to $x_t$). Then, $V(x_t)$ is the optimal cost-to-go at $x_t$, i.e.,
\begin{equation}
\begin{aligned}
    V(x_t) &= \min_{u_t, \cdots, u_{T-1}} \sum_{\tau=t}^{T-1} \hat{c}_t^{\theta}(x_\tau, u_\tau) \\
    &= \sum_{\tau=t}^{T-1} \hat{c}_t^{\theta}(x_{\tau}, u_{\tau}^*)
\end{aligned}
\end{equation}
where $U^* = \crl{u_t^*, u_{t+1}^*, \cdots, x_{T-1}^*}$ is the unique sequence of controls that attains the minimum. Let the corresponding unique sequence of states under the deterministic transition funtion $f$ be $X^* = \crl{x_t, x_{t+1}^*, \cdots, x_{T-1}^*}$. The derivative $\frac{dV(x)}{d\hat{c}_t^{\theta}}$ is
\[
\scaleMathLine{\frac{\partial V(x)}{\partial \hat{c}_t^{\theta}(x_t, u_t)} = 
    \begin{cases}
    1, \text{ if $x_t, u_t$ is a corresponding pair in $X^*\times U^*$}\\
    0, \text{ otherwise. }
    \end{cases}}
\]
A* also returns the optimal cost-to-go $V(x_t) = g(x_t)$ at the current state $x_t$ which is obtained by the same state and control sequences $X^*$ and $U^*$. Therefore, the derivative $\frac{\partial g(x)}{\partial \hat{c}_t^{\theta}(x_t, u_t)}$ is the same as $\frac{\partial V(x)}{\partial \hat{c}_t^{\theta}(x_t, u_t)}$.
\end{proof}

\subsection{Proof of further factorization of $\bfz_t$ into $\bfz_t[k]$}
\begin{proof}
The log odds ratio of the occupancy probability can be expressed as
\begin{equation}
\begin{aligned}
\label{eq:log_odds_proof_forward}
&\log \frac{p(m[j]=1 \mid \bfx_t, \bfz_t)}{p(m[j]=-1 \mid \bfx_t, \bfz_t)} \\
&= \log \frac{p(\bfz_t \mid \bfx_t, m[j]=1) p(m[j]=1 \mid \bfx_t)}{p(\bfz_t \mid \bfx_t, m[j]=-1) p(m[j]=-1 \mid \bfx_t)} \\
&= \sum_{k=1}^K \log \frac{p(z_t[k] \mid \bfx_t, m[j]=1)}{p(z_t[k] \mid \bfx_t, m[j]=-1)} ,
\end{aligned}
\end{equation}
where we have applied Eqn~\eqref{eq:map_prior} \VD{\eqref{eq:map_prior} cannot
  be applied because $p(m[j] = 1 | \bfx_t) \ne p(m[j] = 1)$}
and the independence assumption in each lidar beam~\cite[p152]{Thrun_PR05} in the last equality. We can apply Bayes rule and Eqn~\eqref{eq:map_prior} further to rewrite the forward observation model in Eqn~\eqref{eq:log_odds_proof_forward} as inverse observation model,
\begin{equation}
\begin{aligned}
\label{eq:log_odds_proof_inverse}
&\log \frac{p(m[j]=1 \mid \bfx_t, \bfz_t)}{p(m[j]=-1 \mid \bfx_t, \bfz_t)} \\
&= \sum_{k=1}^K \log \frac{p(m[j]=1 \mid \bfx_t, z_t[k])p(m[j]=1 \mid \bfx_t)}{p(m[j]=-1 \mid \bfx_t, z_t[k])p(m[j]=-1 \mid \bfx_t)} \\
&= \sum_{k=1}^K \log \frac{p(m[j]=1 \mid \bfx_t, z_t[k])}{p(m[j]=-1 \mid \bfx_t, z_t[k])} .
\end{aligned}
\end{equation}
\end{proof}
